# Supplementary material for: PP-Rec: News Recommendation with Personalized User Interest and Time-aware News Popularity
Source: arXiv:2106.01300 source file (2021-06-10)
Supplement: Supplementary file 1 [file Supplement.tex]

\section*{Supplementary Materials}

\subsection*{Experiment Environment}
In this section, we introduce the experiment environment for model training and evaluation.
All experiments listed in this paper are conducted on a server with Ubuntu 16.04.6 operating system.
The server has 6 CPUs whose type is Intel Xeon E5-2690 v4.
The sever has a GPU whose type is Nvidia Tesla P100.
In addition, the memory of the server is 128GB.
We use the Keras (2.2.4) deep learning framework with tensorflow (1.13.0) as backend based on python (3.6) to implement different methods.

\subsection*{Dataset Construction}
We construct two news recommendation datasets from two commercial news platforms.
First, we collect user logs between October 19 and November 15, 2019 from a news website to construct the \textit{NewsWebsite} dataset.
% We show an example news website in Fig.~\ref{fig.website}.
User logs in the last week are used for evaluation, and other user logs are used for model training and validation.
We randomly sample 500k impressions to construct the training dataset, 100k impressions to construct the validation dataset, and 500k impressions to construct the test dataset.
This dataset will be publicly available.

Second, we collect user logs between Jaunary 23 and April 23, 2020 from news feeds to construct the \textit{NewsFeeds} dataset.
% We show an example news feeds in Fig.~\ref{fig.feeds}.
User logs in the last three weeks are used for evaluation, and other user logs are used for model training and validation.
We randomly sample 500k impressions to construct the training dataset, 100k impressions to construct the validation dataset, and 500k impressions to construct the test dataset.

We extract entities from the texts of news titles for each news and linked them to the entities in WikiData\footnote{https://www.wikidata.org/wiki/Wikidata:MainPage} using an entity recognition and linking tool\footnote{This tool is anonymized for double-blind review}.
The knowledge triples including these entities are extracted from WikiData and are further used to train the entity embedding via the transE approach.
The entities and entity embeddings of \textit{NewsWebsite} dataset will be publicly available too.

\subsection*{Data Preprocessing}
We conduct the same preprocessing on the two datasets.
For fair comparisons, all methods are trained and evaluated based on the same processed data.
We construct a word dictionary based on the extracted news titles and filter the words whose occurrence frequency is less than 3.
We split each news title into words and retain the first 30 words.
We randomly sample at most 5 entities for each news.
We use the recent 50 clicked news before the impression start time to construct user click history.

% \begin{figure}
%     \centering
%     \resizebox{0.4\textwidth}{!}{
%     \includegraphics{Src/website.png}
%     }
%     \caption{An example news website.}
%     \label{fig.website}
% \end{figure}

% \begin{figure}
%     \centering
%     \resizebox{0.4\textwidth}{!}{
%     \includegraphics{Src/website.png}
%     }
%     \caption{An example news feeds.}
%     \label{fig.feeds}
% \end{figure}

\begin{table*}[!h]
\centering
\resizebox{0.9\textwidth}{!}{

\begin{tabular}{|c|cccc|cccc|}
\hline
\multirow{2}{*}{Method} & \multicolumn{4}{c|}{NewsWebsites}                                 & \multicolumn{4}{c|}{NewsFeeds}                                    \\ \cline{2-9} 
                        & AUC            & MRR            & nDCG@5         & nDCG@10        & AUC            & MRR            & nDCG@5         & nDCG@10        \\ \hline
ViewNum                 & 55.72$\pm$0.00 & 27.62$\pm$0.00 & 30.15$\pm$0.00 & 37.18$\pm$0.00 & 56.90$\pm$0.00 & 25.31$\pm$0.00 & 28.84$\pm$0.00 & 34.41$\pm$0.00 \\
RecentPop               & 57.37$\pm$0.00 & 29.74$\pm$0.00 & 32.68$\pm$0.00 & 39.14$\pm$0.00 & 56.40$\pm$0.00 & 24.95$\pm$0.00 & 28.37$\pm$0.00 & 33.94$\pm$0.00 \\
CTR                     & 65.41$\pm$0.00 & 34.28$\pm$0.00 & 38.58$\pm$0.00 & 45.56$\pm$0.00 & 66.41$\pm$0.00 & 32.77$\pm$0.00 & 38.43$\pm$0.00 & 43.75$\pm$0.00 \\ \hline
GRU                     & 61.10$\pm$0.02 & 27.65$\pm$0.07 & 29.97$\pm$0.10 & 36.63$\pm$0.01 & 65.10$\pm$0.03 & 28.73$\pm$0.01 & 33.20$\pm$0.02 & 38.92$\pm$0.03 \\
DKN                     & 62.93$\pm$0.47 & 29.11$\pm$0.27 & 31.53$\pm$0.36 & 38.31$\pm$0.29 & 69.33$\pm$0.08 & 33.44$\pm$0.03 & 39.42$\pm$0.03 & 44.74$\pm$0.05 \\
DAN                     & 65.58$\pm$0.40 & 30.62$\pm$0.33 & 33.71$\pm$0.46 & 40.15$\pm$0.37 & 70.39$\pm$0.07 & 34.24$\pm$0.06 & 40.45$\pm$0.07 & 45.76$\pm$0.07 \\
NAML                    & 64.22$\pm$0.71 & 29.78$\pm$0.43 & 32.62$\pm$0.61 & 39.28$\pm$0.47 & 70.09$\pm$0.06 & 33.94$\pm$0.07 & 40.11$\pm$0.07 & 45.44$\pm$0.07 \\
NPA                     & 63.75$\pm$0.19 & 29.24$\pm$0.17 & 32.26$\pm$0.19 & 38.77$\pm$0.18 & 70.23$\pm$0.02 & 34.15$\pm$0.02 & 40.32$\pm$0.03 & 45.65$\pm$0.02 \\
NRMS                    & 65.12$\pm$0.35 & 30.40$\pm$0.39 & 33.40$\pm$0.48 & 40.06$\pm$0.39 & 70.67$\pm$0.03 & 34.46$\pm$0.02 & 40.72$\pm$0.02 & 46.06$\pm$0.02 \\
LSTUR                   & 66.21$\pm$0.20 & 31.06$\pm$0.19 & 34.22$\pm$0.21 & 40.62$\pm$0.16 & 71.09$\pm$0.05 & 34.86$\pm$0.07 & 41.27$\pm$0.07 & 46.55$\pm$0.06 \\ \hline
PP-Rec                & 70.57$\pm$0.09 & 38.76$\pm$0.07 & 44.08$\pm$0.13 & 50.79$\pm$0.11 & 73.14$\pm$0.15 & 35.47$\pm$0.09 & 42.16$\pm$0.10 & 47.13$\pm$0.13 \\ \hline
\end{tabular}

}
\caption{Performance of different approaches on validation datasets. }
\label{table.valid}

\end{table*}

\subsection*{Hyperparameter Settings}
In our experiments, word embeddings are 300-dimensional and initialized by the Glove embeddings~\cite{pennington2014glove}.
The entity embeddings are 100-dimensional vectors pre-trained based on knowledge tuples extracted from WikiData via TransE~\cite{bordes2013translating}.
We use clicked and unclicked impressions in recent one hour to compute the near real-time CTR.
The recency and popularity embedding are set to 100 dimensions and initialized randomly.
All multi-head attention networks are set to have 20 attention heads and the output dimension of each head is 20.
All gate networks are implemented by a two-layer dense network with 100-dimensional hidden vectors.
Besides, two dense networks for calculating content- and recency- based popularity score contain two layers with 128-dimensional vectors. 
All attention networks are based on a two-layer dense network with 100-dimensional hidden vectors to calculate attention weights. 
Dropout approach~\cite{srivastava2014dropout} is applied to \textit{PP-Rec} to migrate overfitting.
The dropout probability is set to 0.2.
Adam~\cite{kingma2014adam} is used for model training with $10^{-4}$ learning rate.
Hyper-parameters of \textit{PP-Rec} and baselines are tuned based on the validation set.
The hyper-parameters used in our approach are summarized in Table~\ref{hyper}.

\begin{table}[h]
\centering
\resizebox{0.8\linewidth}{!}{
\begin{tabular}{|l|c|}
\hline
\multicolumn{1}{|c|}{\textbf{Hyperparameters}}& \textbf{Value} \\ \hline
word embedding dimension                     & 300            \\
entity embedding dimension                  & 100 \\
CTR embedding dimension                  & 100 \\
recency embedding dimension                  & 100 \\
\# heads of multi-head attention networks                 & 20             \\
output dim of attention head               & 20            \\
dim of attention query             & 200            \\
dropout ratio                       & 0.2            \\
optimizer                                    & Adam           \\
learning rate                                & 1e-4           \\
batch size                                   & 32    \\     
training epoch                                   & 2    \\  

\hline
\end{tabular}
}
\caption{Detailed settings of hyperparameters.}\label{hyper}
\end{table}

\subsection*{Model Computational Cost}

There are 19.6M parameters in the \textit{PP-Rec} model except for the word and entity embedding layer.
There are 12.2M parameters in the word embedding layer and 2.7M parameters in the entity embedding layer in the \textit{NewsWebsite} dataset.
There are 33.6M parameters in the word embedding layer and 29.9M parameters in the entity embedding layer in the \textit{NewsFeeds} dataset.
It takes 4,473 seconds to train \textit{PP-Rec} for one epoch on the \textit{NewsWebsite} dataset.
It takes 3,312 seconds to train \textit{PP-Rec} for one epoch on the \textit{NewsFeeds} dataset.

\subsection*{Evaluation Metric}

In this section, we introduce the evaluation metric we used in detail.
Denotes $\mathcal{N}_p$ as the set of clicked news articles and $\mathcal{N}_n$ as the set of non-clicked news articles in an impression.
Denotes $R(\cdot)$ as the ranked position of the sample $\cdot$.
\begin{equation*}
    \begin{split}
        &AUC=\frac{\sum\limits_{p_i \in \mathcal{N}_p }\sum\limits_{ n_j \in \mathcal{N}_n  } I(R(p_i)<R(n_j))}{ |\mathcal{N}_p|*|\mathcal{N}_p|  },\\
        &MRR=\frac{1}{ |\mathcal{N}_p| }\sum_{ p_i \in \mathcal{N}_p } \frac{1}{R(p_i)},\\
        &nDCG@K=\frac{\sum_{i=1}^{K}(2^{r_i}-1)/\log_2(1+i)}{ \sum_{i=1}^{ |\mathcal{N}_p| }1/\log_2(1+i)},
    \end{split}
\end{equation*}
$I(\cdot)$ is the indicator function and $r_i$ denotes the relevance label of the news article ranked in the $i$-th position.
The relevance label is 1 for the clicked news article and 0 for the non-clicked news article.
The implement of these metrics is in the python file utils.py (line 28 - line 60) in the uploaded code.

\subsection*{Validation Performance}
We summarized the performance of different approaches on the validation sets in Table~\ref{table.valid}.
The hyper-parameters are selected based on the AUC performance of models on the validation dataset.
We select hyper-parameters by manual tunning.

\subsection*{Effect of Popularity on User Modeling}

We conduct experiments to evaluate the effectiveness of news popularity for user interest modeling.
The experimental results are shown in Fig.~\ref{fig.exp.user_encoder}.
We find that after removing news popularity for user modeling, the performance of \textit{PP-Rec} declines significantly.
This is because news popularity usually influences users' click behaviors, which may cause bias in users' historical clicks.
Eliminating news popularity bias can help model user interests more accurately.
Thus, removing news popularity for user modeling makes \textit{PP-Rec} cannot effectively model the relative importance of clicked news for user interest modeling and hurts the recommendation accuracy.

% \begin{figure}
% \centering
% \begin{minipage}{0.23\textwidth}
%   \centering
% \resizebox{\textwidth}{!}{  \includegraphics{Src/user_encoder.pdf}}
%   \caption{Effect of popularity on user modeling.}
%   \label{fig.exp.user_encoder}
% \end{minipage}\hfill
% \begin{minipage}{0.23\textwidth}
%   \centering
% \resizebox{\textwidth}{!}{  \includegraphics{Src/news_encoder.pdf}}
%   \caption{Effect of knowledge on news modeling}
%   \label{fig.exp.news_encoder}
% \end{minipage}
%     %\%\vspace{-0.2in}

% \end{figure}

\begin{figure}
    \centering
    \resizebox{0.3\textwidth}{!}{
    \includegraphics{Src/user_encoder.pdf}
    }
    \caption{Effect of popularity on user modeling.}
    \label{fig.exp.user_encoder}
\end{figure}

\subsection*{Effect of Knowledge on News Modeling}

\begin{figure}
    \centering
    \resizebox{0.3\textwidth}{!}{
    \includegraphics{Src/news_encoder.pdf}
    }
    \caption{Effect of knowledge on news modeling.}
    \label{fig.exp.news_encoder}
\end{figure}

We evaluate the effectiveness of knowledge for news content modeling by removing the components related to entities in \textit{knowledge-aware news encoder}.
The experimental results are summarized in Fig.~\ref{fig.exp.news_encoder}. 
We find that removing the knowledge used for news content modeling hurts the performance.
This is because knowledge contains some information that is related to news content and beyond the text information.
For example, given two news titles, i.e., `` `Cats': it's not about actors'' and `` Taylor Swift sells her favorite jets'', it is difficult to capture the relatedness between the two news articles from the texts of their titles.
However, entities can incorporate the knowledge that Taylor is the actor of the film 'Cats', which can help model capture the relatedness between the two news articles.
Thus, removing the knowledge hurts the accuracy of news content modeling and hurts the accuracy of recommendation.
